# Supplementary material for: History by Diversity: Helping Historians search News Archives
Source: arXiv:1810.10251 source file (2018-10-24)
Supplement: Supplementary file 1 [file appendix.tex]

\section*{Appendix: Tables}

\paragraph{robustness}
Once the pools were evaluated, a standard robustness test was carried out with TIA-SBR as the primary measure. We selected 25\% of the query workload at random and split them into two equal sets. We selected 50\% of the runs at random for retrieval depth 10 and calculated ranked the system runs for both sets of queries. We found that the rankings were consistent for p<=0.05.

\begin{table*}[!t]
  \small
  \centering
  \scalebox{0.75}{
  \begin{tabular}{@{}rccllllllllllll@{}}\toprule
    %\multicolumn{2}{c}{} & \multicolumn{3}{c}{\textbf{GRD}} && \multicolumn{3}{c}{\textbf{APX}} && \multicolumn{3}{c}{\textbf{OPT}}\\
    %\cmidrule{3-5} \cmidrule{7-9}\cmidrule{11-13}
    \multicolumn{2}{l}{} && \textsc{Sbr} && \textsc{TIA-Ndcg} &&  \textsc{TIA-Prec.} && \textsc{TIA-Map} && \textsc{TIA-Err} && \textsc{TIA-SBR} \\ \midrule

    \multicolumn{2}{l}{\textbf{LM}}&& 0,391 && 0,109 && 0,009 && 0,01 &&  0,026 && 0,544     \\

    \multicolumn{2}{l}{\textbf{T-IA-Select}}&& 0,447 && 0,131 && 0,009 && 0,011 &&  0,031 && 0,58     \\

    \multicolumn{2}{l}{\textbf{T-PM2}} && 0,25 && 0,061 && 0,01 && 0,012 &&  0,023 && 0,408     \\

    \multicolumn{2}{l}{\textbf{IA-Select}} && 0,382 && 0,11 && 0,009 && 0,009 && 0,023 && 0,526   \\

    \multicolumn{2}{l}{\textbf{PM2}} && 0,381 && 0,107 && 0,01 && 0,011 && 0,028 && 0,526      \\

    \multicolumn{2}{l}{\textbf{MDIV}} && 0,401 && 0,115 && 0,01 && 0,01 &&  0,027 && 0,563     \\

    \multicolumn{2}{l}{\textbf{LM+t+D}} && 0,481 && 0,134 && 0,006 && 0,009 && 0,026 && 0,603     \\

    \multicolumn{2}{l}{\textbf{HistDiv}} && 0,48 && 0,151 && 0,009 && 0,011 &&  0,034 && 0,637 \\
    \bottomrule
  \end{tabular}}
  \caption{Retrieval Effectiveness ($k$ = 20)}
  \label{tab:retrireval-effectiveness}
\end{table*}

\begin{table*}[!t]
  \small
  \centering
  \begin{tabular}{@{}rcccccccccccccc@{}}\toprule
    %\multicolumn{2}{c}{} & \multicolumn{3}{c}{\textbf{GRD}} && \multicolumn{3}{c}{\textbf{APX}} && \multicolumn{3}{c}{\textbf{OPT}}\\
    %\cmidrule{3-5} \cmidrule{7-9}\cmidrule{11-13}
    \multicolumn{2}{l}{} && \textsc{Sbr} && \textsc{Ndcg} &&  \textsc{IA-Prec.} && \textsc{Map} && \textsc{Ia-Err} && \textsc{TIA-SBR} \\ \midrule

    \multicolumn{2}{l}{\textbf{LM}} && 0,302 && 0,466 && 0,01 && 0,01 && 0,023 && 0,453       \\

    \multicolumn{2}{l}{\textbf{T-IA-Select}} &&0,325 && 0,479 && 0,01 && 0,012 && 0,028 && 0,456      \\

    \multicolumn{2}{l}{\textbf{T-PM2}} && 0,182 && 0,242 && 0,011 && 0,012 && 0,022 && 0,322     \\

    \multicolumn{2}{l}{\textbf{IA-Select}} && 0,258 && 0,399 && 0,008 && 0,009 && 0,02 && 0,376    \\

    \multicolumn{2}{l}{\textbf{PM2}} && 0,295 && 0,429 && 0,011 && 0,011 && 0,025 && 0,444     \\

    \multicolumn{2}{l}{\textbf{MDIV}} && 0,309 && 0,479 && 0,009 && 0,011 && 0,025 && 0,454     \\

    \multicolumn{2}{l}{\textbf{LM+t+D}} && 0,344 && 0,507 && 0,007 && 0,01 && 0,024 && 0,482     \\

    \multicolumn{2}{l}{\textbf{HistDiv}} && 0,351 && 0,624 && 0,01 && 0,012 && 0,031 && 0,519     \\
    \bottomrule
  \end{tabular}
  \caption{Retrieval Effectiveness ($k$ = 10)}
  \label{tab:retrireval-effectiveness}
\end{table*}

% Please add the following required packages to your document preamble:
% \usepackage{booktabs}
% Please add the following required packages to your document preamble:
% \usepackage{booktabs}
\begin{table}[h]
\begin{tabular}{@{}lllll@{}}
\toprule
 & 5 & 10 & 15 & 20 \\ \midrule
t-pm2 & 0,243 & 0,323 & 0,376 & 0,409 \\
t-iasel & 0,325 & 0,453 & 0,525 & 0,574 \\
mdiv & 0,35 & 0,436 & 0,52 & 0,555 \\
lm & 0,318 & 0,451 & 0,502 & 0,54 \\
lm+t+d & 0,362 & 0,481 & 0,569 & 0,605 \\
asptd & \textbf{0,376} & \textbf{0,518} & \textbf{0,577} & \textbf{0,641} \\ \bottomrule
\end{tabular}
\end{table}

\begin{table*}[!t]
  \small
  \centering
  \begin{tabular}{@{}rcccccccccccccc@{}}\toprule
    %\multicolumn{2}{c}{} & \multicolumn{3}{c}{\textbf{GRD}} && \multicolumn{3}{c}{\textbf{APX}} && \multicolumn{3}{c}{\textbf{OPT}}\\
    %\cmidrule{3-5} \cmidrule{7-9}\cmidrule{11-13}
    \multicolumn{2}{l}{} && \textsc{5} && \textsc{10} &&  \textsc{15} && \textsc{20} \\ \midrule

    \multicolumn{2}{l}{\textbf{LM}} && 0,318 && 0,451 && 0,502 && 0,54           \\

    \multicolumn{2}{l}{\textbf{T-IA-Select}} && 0,325 && 0,453 && 0,525 && 0,574      \\

    \multicolumn{2}{l}{\textbf{T-PM2}} && 0,243 && 0,323 && 0,376 && 0,409     \\

    \multicolumn{2}{l}{\textbf{MDIV}} && 0,35 && 0,436 && 0,52 && 0,555      \\

    \multicolumn{2}{l}{\textbf{LM+t+D}} && 0,362 && 0,481 && 0,569 && 0,605      \\

    \multicolumn{2}{l}{\textbf{HistDiv}} && \textbf{0,376} && \textbf{0,518} && \textbf{0,577} && \textbf{0,641}      \\
    \bottomrule
  \end{tabular}
  \caption{Retrieval Effectiveness ($k$ = 10)}
  \label{tab:retrireval-effectiveness}
\end{table*}

% Please add the following required packages to your document preamble:
% \usepackage{booktabs}
% \usepackage{graphicx}
\begin{table*}[!t]
  \small
  \centering
\begin{tabular}{@{}rccccccc@{}}\toprule

\multicolumn{2}{l}{}                   && sbr    && ndcg   && ia-pr  && map    && ia-err && TIA-SBR && nn   \\ \midrule
\multicolumn{2}{l}{\textbf{PM2}}       && 0.0075 && 0.0439 && 0.0047 && 0.0769 && 0.1115 && 0.0072 && 0.8503 \\ \midrule
\multicolumn{2}{l}{\textbf{HistDiv}}   && 0.0044 && 0.2169 && 0.0128 && 0.1923 && 0.2459 && 0.0053 && 0.7268 \\ \bottomrule
\end{tabular}
\caption{Results for \emph{summer olympics doping scandals}}
\label{table:olympics}
\end{table*}

k=10
methods --  sbr  ndcg  ia-precision  map  ia-err  ta-sbr 
iasel 0,326 && 0,217 && 0,01 && 0,011 && 0,028 && 0,456 && 
pm2 0,182 && 0,108 && 0,011 && ? && 0,021 && 0,321 && 
mdiv 0,313 && 0,216 && 0,009 && 0,01 && 0,025 && 0,462 && 
ntpm2 0,296 && 0,196 && 0,01 && ? && 0,025 && 0,446 && 
lm 0,306 && 0,212 && 0,01 && 0,01 && 0,023 && 0,458 && 
masptd 0,347 && 0,272 && 0,01 && 0,012 && 0,031 && 0,512 && 
ntiasel 0,259 && 0,163 && 0,008 && 0,009 && 0,02 && 0,376 && 
lm+t+d 0,346 && 0,227 && 0,007 && 0,009 && 0,024 && 0,484 && 
masptdhard 0,357 && 0,274 && 0,01 && 0,012 && 0,031 && 0,525 &&

k=20
methods --    sbr  ndcg  ia-precision  map   ia-err  ta-sbr 
iasel  && 0,447 && 0,131 && 0,009 && 0,011 &&  0,031 && 0,58
pm2  && 0,25 && 0,061 && 0,01 && 0,012 &&  0,023 && 0,408 
mdiv && 0,401 && 0,115 && 0,01 && 0,01 &&  0,027 && 0,563 
ntpm2 && 0,381 && 0,107 && 0,01 && 0,011 && 0,028 && 0,526 
lm  && 0,391 && 0,109 && 0,009 && 0,01 &&  0,026 && 0,544 && 
masptd  && 0,48 && 0,151 && 0,009 && 0,011 &&  0,034 && 0,637 
ntiasel  && 0,382 && 0,11 && 0,009 && 0,009  0,023 && 0,526 && 
lm+t+d  && 0,481 && 0,134 && 0,006 && 0,009 && 0,026 && 0,603 &&

1d measures:
methods --  ia-precision1d  sbr1d  ia-err1d  ndcg1d  map1d 
iasel 0,171 && 0,632 && 0,323 && 0,281 && 0,195 && 
pm2 0,176 && 0,524 && 0,285 && 0,222 && ? && 
mdiv 0,17 && 0,676 && 0,331 && 0,296 && 0,191 && 
ntpm2 0,183 && 0,67 && 0,309 && 0,293 && ? && 
lm 0,179 && 0,686 && 0,317 && 0,311 && 0,194 && 
masptd 0,163 && 0,711 && 0,331 && 0,317 && 0,19 && 
ntiasel 0,142 && 0,555 && 0,255 && 0,247 && 0,163 && 
lm+t+d 0,144 && 0,695 && 0,316 && 0,282 && 0,174 && 
masptdhard 0,169 && 0,732 && 0,335 && 0,329 && 0,191 &&
